# Supplementary material for: Grey Literature in Software Engineering: A Critical Review
Source: arXiv:2104.13435 source file (2021-05-12)
Supplement: Supplementary file 1 [file appendixB.tex]

\appendix{Appendix B: Secondary Studies Included}\label{appendixSecondaryStudiesIncluded}

\scriptsize{
\begin{longtable}{lccclr}
\caption{Selected Secondary Studies} \\
\label{tab:secondaryStudies}

\textbf{Study ID}
& \textbf{Year}
& \textbf{Source Type}
& \textbf{Review Type}
& \textbf{Search Method}
& \textbf{\% of GL} \\

\hline

\endhead

\hline
\multicolumn{6}{l@{}}{\textbf{Source Type:} J -- Journal; C -- Conference.} \\
\multicolumn{6}{l@{}}{\textbf{Review Type:} SLR -- Systematic Literature Review; MLR -- Multivocal Literature Review;} \\
\multicolumn{6}{l@{}}{MS -- Mapping Study; GL -- Grey Literature} \\
\multicolumn{6}{l@{}}{\textbf{Search Method:} A -- Automatic; M -- Manual; S - Snowballing.} \\
\hline

\endfoot

SC2468 & 2018 & J & SLR & A & 12.9 \\ 

MS-EASE-158 &2016& C & SLR & A & 4.5 \\ 

SC443 &2015& J & SLR & A & 2.3 \\ 

SC465 &2016& J & SLR & A + M & 6.5 \\ 

MS-IST-797 &2015& J & SLR & A + S & 12.6 \\ 

SC2340 &2018& J & MS & A & 4.4 \\ 

MS-IST-534 &2015& J & MS & A + M + S & 7.8 \\ 

SC67 &2015& J & SLR & A & 19.0 \\ 

MS-IST-598 &2017& J & SLR & A & 23.8 \\ 

MS-TSE-535 &2017& J & Others & A & 5.3 \\ 

MS-JSS-890 &2017& J & Others & A + M + S & 12.4 \\ 

MS-TSE-481 &2016& J & SLR & A & 2.5 \\ 

SC6555 &2018& J & MS & A + M & 1.3 \\ 

SC3398 &2018& J & SLR & A + M & 3.6 \\ 

SD274 &2015& J & SLR & A + M & 13.8 \\ 

MS-IST-815 &2015& J & SLR & A + M & 0 \\ 

MS-JSS-776 &2015& J & SLR & A + S & 25.9 \\ 

MS-IST-407 &2015& J & SLR & A & 2.3 \\ 

MS-IST-543 &2017& J & SLR & A + M & 20.4 \\ 

SC3386 &2018& J & SLR & A + M + S & 6.3 \\ 

SC542 &2016& J & SLR & A + S & 1.6 \\ 

MS-JSS-1513 &2015& J & MS & A + M + S & 10.1 \\ 

SC3464 &2018& J & MS & A + M + S & 7.5 \\ 

MS-JSS-1477 &2016& J & MS & A & 2.5 \\ 

MS-JSS-661 &2015& J & MS & A & 68.4 \\ 

MS-IST-816 &2015& J & SLR & A + M + S & 22.6 \\ 

MS-IST-652 &2015& J & MS & A & 6.9 \\ 

MS-IST-355 &2015& J & MS & A + M & 6.7 \\ 

MS-IST-749 &2017& J & SLR & A + S & 3.1 \\ 

MS-IST-807 &2015& J & SLR & A + M & 2.3 \\ 

MS-ESE-286 &2017& J & SLR & A & 20.0 \\ 

MS-IST-608 &2015& J & SLR & A + M & 0 \\ 

MS-ESE-141 &2015& J & MS & A & 4.0 \\ 

SC2329 &2018& J & MLR & A & 41.7 \\ 

SC3080 &2018& C & SLR & A + S &100 \\ 

MS-IST-726 &2015& J & SLR & A + M & 8.6 \\ 

MS-EASE-97 &2014& C & SLR & A + M & 5.6 \\ 

ACM347 &2014& J & MS & A + M & 7.1 \\ 

MS-IST-519 &2014& J & SLR & A + M + S & 1.5 \\ 
MS-JSS-1323 &2017& J & SLR & A + S & 3.3 \\ 

SC653 &2016& J & SLR & A & 10.0 \\ 

MS-EASE-170 &2016& C & SLR & A + S & 100 \\ 

MS-JSS-396 &2016& J & SLR & A & 5.8 \\ 

SC2845 &2018& J & SLR & A + S & 1.9 \\ 

MS-IST-375 &2014& J & MS & A & 4.2 \\ 

MS-JSS-900 &2017& J & Others & A + M &100 \\ 

NETO-2019-S1 &2017& C & GL & A & 100 \\ 

MS-JSS-1229 &2014& J & SLR & A & 2.2 \\ 

SC1799 &2018& J & SLR & A + S & 30.1 \\ 

MS-IST-541 &2014& J & SLR & A + M + S & 8.2 \\ 
MS-TSE-303 &2014& J & SLR & A + M + S & 4.5 \\ 
MS-IST-214 &2017& J & MS & A + S & 5.6 \\ 

MS-IST-624 &2014& J & MS & A + M + S & 7.7 \\ 

MS-IST-757 &2016& J & MS & A + S & 0 \\ 

SC2433 &2018& J & SLR & A & 2.6 \\ 

SC1873 &2018& J & SLR & A + S & 63.2 \\ 

MS-IST-462 &2014& J & SLR & A + S & 3.2 \\ 

MS-ESE-190 &2014& J & SLR & A + M & 45.9 \\ 

SC2622 &2018& J & Others & A + S & 7.7 \\ 

MS-IST-370 &2014& J & MS & A & 4.8 \\ 

MS-ESEM-238 &2014& J & MS & A + S & 4.4 \\ 

MS-JSS-349 &2016& J & MS & A & 36.0 \\ 

SC470 &2013& C & MS & A + M + S & 1.6 \\ 

SC221 &2016& C & MS & A + M + S & 7.5 \\ 

SC3363 &2018& J & SLR & A + S & 0 \\ 

MS-JSS-463 &2017& J & MS & A + S & 7.9 \\ 

MS-JSS-1279 &2013& J & MLR & A & 39.1 \\ 

MS-IST-321 &2017& J & MS & A + S & 7.5 \\ 

MS-IST-522 &2013& J & MS & A + M & 1.8 \\ 

MS-IST-582 &2013& J & MS & A + M & 12.3 \\ 

MS-IST-688 &2013& J & SLR & A + S & 5.0 \\ 

MS-JSS-1527 &2018& J & SLR & A + S & 4.8 \\ 

SC2603 &2018& J & SLR & A + M & 9.7 \\ 

MS-JSS-784 &2013& J & SLR & A + S & 8.5 \\ 

MS-IST-680 &2013& J & SLR & A + M & 0 \\ 

MS-IST-331 &2017& J & MS & A + M & 11.5 \\ 

MS-IST-675 &2013& J & SLR & A + S & 15.1 \\ 

MS-JSS-167 &2016& J & MS & A + M & 16.7 \\ 

MS-IST-343 &2017& J & MS & A + S & 3.7 \\ 

MS-ESE-337 &2017& J & MS & A + S & 7.6 \\ 

MS-EASE-22 &2012& C & MS & A & 27.6 \\ 

MS-TSE-538 &2017& J & SLR & A + S & 1.8 \\ 

SC2905 &2018& J & SLR & A & 13.9 \\ 

MS-IST-419 &2012& J & SLR & A + S & 2.7 \\ 

MS-IST-288 &2012& J & SLR & A + M & 18.9 \\ 

MS-IST-193 &2012& J & SLR & A & 6.1 \\ 

SC2312 &2018& J & SLR & A + S & 0.9 \\ 

SC7064 &2018& J & MS & A & 0 \\ 

SC166 &2012& J & SLR & A & 17.9 \\ 

SC3282 &2018& J & MLR & A + S & 80.1 \\ 

MS-JSS-108 &2016& J & MS & A & 3.6 \\ 

MS-JSS-683 &2017& J & SLR & A + S & 2.1 \\ 

MS-IST-574 &2012& J & SLR & A & 3.6 \\ 

MS-EASE-47 &2012& C & SLR & A + S & 0 \\ 

MS-IST-711 &2012& J & SLR & A & 13.8 \\ 

MS-EASE-40 &2012& C & SLR & A + M & 0 \\ 

SC2601 &2018& J & MS & A + M + S & 7.4 \\ 

MS-IST-354 &2017& J & MLR & A & 28.2 \\ 

SC2922 &2018& J & MLR & A + S & 73.0 \\ 

SC3100 &2018& C & Others & M & 12.5 \\ 

MS-IST-476 &2017& J & SLR & A & 7.1 \\ 

MS-JSS-622 &2016& J & SLR & A & 4.2 \\ 

SC1168 &2016& J & SLR & A + S & 0.8 \\ 

MS-ESEM-72 &2012& J & Others & A & 9.1 \\ 

MS-JSS-1224 &2017& J & MS & A + M + S & 0.3 \\

MS-IST-754 &2016& J & SLR & A & 5.7 \\ 

MS-IST-246 &2011& J & MS & A + S & 4.4 \\ 

MS-ESEM-07 &2011& J & MS & A + M & 15.4 \\ 

SD288 &2011& J & SLR & A + M & 1.0 \\ 

SC91 &2011& J & SLR & A + M & 5.0 \\ 

MS-EASE-02 &2011& C & MS & A + M + S & 8.8 \\ 

MS-EASE-194 &2016& C & MLR & A & 28.2 \\ 

SC5968 &2018& J & GL & A & 100 \\ 

IEEE63 &2011& C & SLR & A & 12.5 \\ 

MS-JSS-437 &2011& J & Others & A + S & 18.8 \\ 
MS-TSE-16 &2011& J & SLR & A & 6.8 \\ 

MS-JSS-695 &2011& J & SLR & A & 13.9 \\ 

MS-JSS-728 &2017& J & MS & A & 40.8 \\ 

MS-EASE-12 &2011& C & SLR & A + M & 2.9 \\ 

MS-TSE-09 &2011& J & SLR & A + M + S & 3.8 \\ 

MS-IST-632 &2011& J & MS & A + M & 6.1 \\ 

SC2965 &2018& C & GL & A &100 \\ 

CRUZES-2011-S22 &2010& J & MS & A + M + S & 31.6 \\ 

CRUZES-2011-S46 &2010& J & SLR & A & 1.4 \\ 

CRUZES-2011-S33 &2010& J & MS & A + M + S & 2.5 \\ 

MS-IST-353 &2016& J & MLR & A & 66.7 \\  \\ 

\end{longtable}
}

\noindent{\large\bfseries Included Secondary Studies References\par}
%\subsection{References}

\nocitesec{*}
%\bibliographystylesec{elsarticle-num}
\bibliographystylesec{appendixStyle}
\bibliographysec{secondaryStudies}
