# Supplementary material for: Grey Literature in Software Engineering: A Critical Review
Source: arXiv:2104.13435 source file (2021-05-12)
Supplement: Supplementary file 2 [file appendixA.tex]

\appendix{Appendix A: Secondary Studies without GL}\label{appendix-secondar-studies-without-gl}

%\noindent{\large\bfseries Included Secondary Studies References\par}
%\subsection{References}

\nocitesec{*}
%\bibliographystylesec{elsarticle-num}
\bibliographystylesec{appendixStyle}
\bibliographysec{secondaryStudiesNotIncluded}
